# Supplementary material for: Generalizable Neural Human Renderer
Source: arXiv:2404.14199 source file (2024-04-22)
Supplement: Supplementary file 1 [file supp_ablation.tex]

\begin{table}[tb]
    \centering
    \captionsetup{aboveskip=0pt}\captionsetup{belowskip=0pt}
    \caption{Additional Ablations and comparisons. Our final model is underlined.}
    \scalebox{0.87}{
    \begin{tabular}{llccccc}
    \Xhline{3\arrayrulewidth}
                    \multicolumn{1}{c}{Experiment}              & \multicolumn{1}{c}{Method}  & PSNR$\uparrow$ & SSIM$\uparrow$ & LPIPS$\downarrow$ & \multicolumn{2}{c}{Avg. $\downarrow$}  \\ \hline \hline
        \multirow{4}{*}{Feat dim of $\Phi_\text{multi\_frame}$} & 32 & 27.26 & 0.962  & 42.64 & 24.93 & (+0.) \\
                                    & 64 & 27.30 & 0.962  & 43.46 & 25.04 & (+5.99) \\
                                    & 128 & 27.45 & 0.962 & 41.77 & 24.41 & (+0.35) \\
                                    & \ul{256} & 27.24 & 0.963 & 42.00 & 24.81  &  (+0.86) \\ \hline 
        \multirow{3}{*}{Depth of $\Phi_\text{multi\_frame}$}& 2 & 27.32 & 0.961 &  41.91 & 24.56 & (+0.61) \\
                                    & 3 & 26.45 & 0.956  & 56.71 & 29.94 & (+5.99) \\
                                     & \ul{4} & 24.84 & 0.954 & 51.79 & 33.25 &  (+9.30)\\ 
        \hline
    \end{tabular}}
    \label{tab:supp_ablation}
\end{table}
